# Supplementary material for: Normalize Then Propagate: Efficient Homophilous Regularization for Few-shot Semi-Supervised Node Classification
Source: arXiv:2501.08581 source file (2025-01-15)
Supplement: Supplementary file 1 [file appendix.tex]

\section{Appendix}
% \section{Appendix / supplemental material}

\subsection{Hyperspherical Prototype}
\label{sec:hpn}
As a classic approach, prototype-based methods focus on capturing the distance between a given example $x$ and prototypes, where each prototype has an associated class label. $x$ is then assigned to the class of the closest prototype.
In the case of Prototypical Networks \cite{nips2017prototypical-network}, the prototype layer generates a distribution over classes for a given example $x$ by applying a softmax function to distances between the prototypes and $f_\phi(x)$ in the embedding space:
\begin{equation}
\label{eq:prototype-net}
    p_\phi ( y = k \; \big| \; x ) = \frac{
        \mathrm{exp} \left( -d ( f_\phi(x) \; , \; P_k ) \right)
    }{
        \sum_{k' \in \mathcal{C}} \mathrm{exp} \left( -d ( f_\phi (x) \; , \; P_{k'} ) \right)
    } \quad , 
\end{equation}
where $P_k$ denotes the prototype of class $k$; $d(\cdot)$ denotes distance metric; $\mathcal{C} = \{ c_1, c_2, \cdots , c_L \}$ denotes the labels.
A common approach is to define prototypes as the mean output vector over training examples per class, e.g. , $P_k = \frac{1}{|S_k|} \sum_{ (x_i, y_i) \in S_k } f_\phi (x_i)$, where $(x_i, y_i)$ denotes training example and its label; $S_k$ denotes the training set.
In this paper, we utilize class prototypes that are defined a priori with large margin separation from Hyperspherical Prototype Network \cite{nips2019hpn}.

% The optimization hinges on the presence of class prototypes that devide the output space prior to learning. Rather than relying on one-hot vector, which only use the postive portion of the output space and require at least as many dimensions as classes, we incorporate the inductive biases of large margin sparation and simplicity.
In order to obtain the predefined hyperspherical prototype with a large margin separation, we aim to distribute the prototypes as uniformly as possible on the hypersphere.
In geometry, the problem mentioned above, known as the Tammes problem~\cite{musin2015tammes-problem}, involves the challenge of distributing $C$ points uniformly on a unit hypersphere to maximize the minimum distance between any two points.
% \begin{equation}
% \label{eq:prototypes-optim}
%     \mathbf{P}^* = \operatorname*{arg\,min}_{\mathbf{P}' \in \mathbb{P}}
%     \left(
%         \operatorname*{max}_{\left( k, l, k \neq l \right) \in C} \mathop{cos} \theta_{ \left( \mathbf{p}_k' , \mathbf{p}_l' \right)}
%     \right)
% \end{equation}
We adopt the concise optimization method proposed in the Hypershperical Prototype Networks \cite{nips2019hypersphericalProtoNet} for determining the data-independent hyperspherical prototypes:
\begin{equation}
 \label{eq:hyper-prototype-optim}
    \mathcal{L}_\mathrm{HP} = \frac{1}{K} \sum_{i = 1}^K \operatorname*{max}_{j \in C} \left(
        \hat{\mathbf{P}} \hat{\mathbf{P}}^\mathrm{T} - 2\mathbf{I}
    \right)_{ij}
    \; , \;
    \text{s.t.} \; \forall \, \big\Vert \, \hat{\mathbf{P}} \, \big\Vert = 1 \; .
\end{equation}

\subsection{Details of Datasets}
\label{sec:data-detail}
Cora, Citeseer, Pubmed (Planetiod datasets)\cite{icml2016planetoid-dataset}, and Cora-ML are extensively utilized citation networks.
MS-CS\cite{shchur2018pitfalls}, based on the Microsoft Academic Graph, is a co-authorship network.
The detailed statistics of these datasets are listed in Table \ref{tab:dataset}, while the calculation method for homophily is outlined as follows:
\begin{equation}
\label{eq:homophily-def}
    h = \frac{1}{| V |} \sum_{i \in V} \left( \frac{ \sum_{j \in \mathcal{N}_i } \mathbf{1} \left( y_i, y_j \right) } { |\mathcal{N}_i| } \right) \; ,
\end{equation}
where $h$ is defined as the average ratio of neighborhoods with the same label as the center node \cite{iclr2020geom-gcn}.
For the standard semi-supervised node classification, we follow the previous works \cite{DBLP:conf/iclr/2017/gcn, icml2022gcnii, ijcai2023violin}, with the 20 labeled nodes per class.
For the few-shot semi-supervised node classification, we follow the settings of Meta-PN \cite{aaai2022meta-pn}.
Moreover, for the ogbn-arxiv dataset, we randomly select 2.5\% of the nodes from the training set as labeled data, while maintaining the same validation and test splits as defined in the OGB Benchmark \cite{hu2020ogb}.
We conducted 10 random splits on ogbn-arxiv, which can be found in the supplementary materials.

\begin{table}
    \centering
    \resizebox{\linewidth}{!}{
        \begin{tabular}{lrrrrrrrr}
        \toprule
        Dataset     & Cora      & Citeseer  & Pubmed    & Cora-ML   & MS-CS     & ogbn-arxiv\\
        \midrule
        \#Nodes     & 2,708     & 3,327     & 19,717    & 2,995     & 18,333    & 169,343   \\
        \#Edges     & 5,429     & 4,732     & 44,338    & 8,158     & 1,166,243 & 2,315,598 \\
        \#Features  & 1,433     & 3,703     & 500       & 2,879     & 6,805     & 128       \\
        \#Classes   & 7         & 6         & 3         & 7         & 15        & 40        \\
        Degree      & 3.9       & 2.8       & 4.5       & 5.5       & 4.5       & 7.7       \\
        Homophily   & 0.83      & 0.72      & 0.79      & 0.81      & 0.83      & 0.63      \\
        \bottomrule
        \end{tabular}
    }
\caption{Brief Statistics of datasets}
\label{tab:dataset}
\end{table}
% \begin{figure}
%   \begin{minipage}[b]{.45\linewidth}
%     \centering
%     \includegraphics[width=0.7\linewidth]{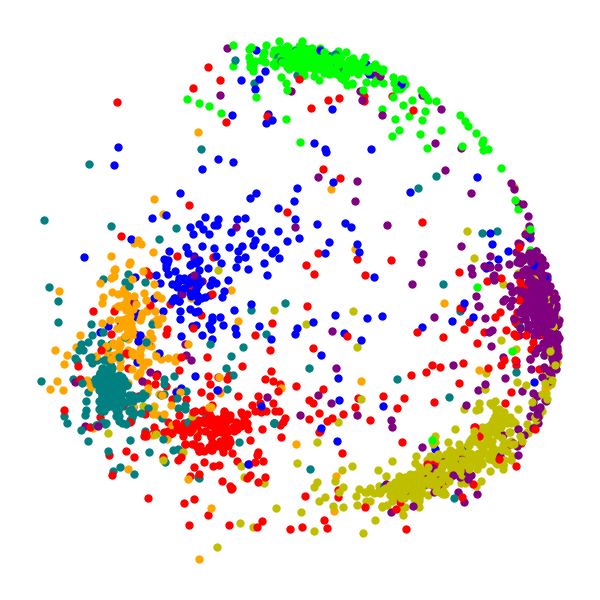}
%     % \captionof{figure}{Figure caption}% \caption{Figure caption}
%     \caption{Image}
%   \end{minipage}\hfill
%   \begin{minipage}[b]{.45\linewidth}
%     \centering
%     \begin{tabular}{ *{5}{c} }
%       A & b & C & d & e \\
%       \hline
%       1 & 2 & 3 & 4 & 5
%     \end{tabular}
%     % \captionof{table}{Table caption}
%     \caption{Table}
%   \end{minipage}
% \end{figure}

\subsection{Visualization}
\label{sec:tsne}
In Figure \ref{fig:tsne-planetoid} we show the visualization on Planetoid datasets using the representations generated by NormProp from different layers. We employ the t-SNE \cite{van2008tsne} method for dimensionality reduction.
According to the Figure \ref{fig:tsne-planetoid}, we can visually observe the evolution of the node from the unit hypersphere to its final representations.

\begin{figure}[H]
    \centering
    \begin{minipage}[b]{\linewidth}
        \centering
        \subfigure[Cora $Z^{(0)}$]{
            \centering
            \includegraphics[width=0.3\linewidth]{resources/visual_cora0.png}
            \label{fig:tsne-cora0}
        }
        % \hspace{0.06\textwidth}
        \subfigure[Cora $Z^{(1)}$]{
            \centering
            \includegraphics[width=0.3\linewidth]{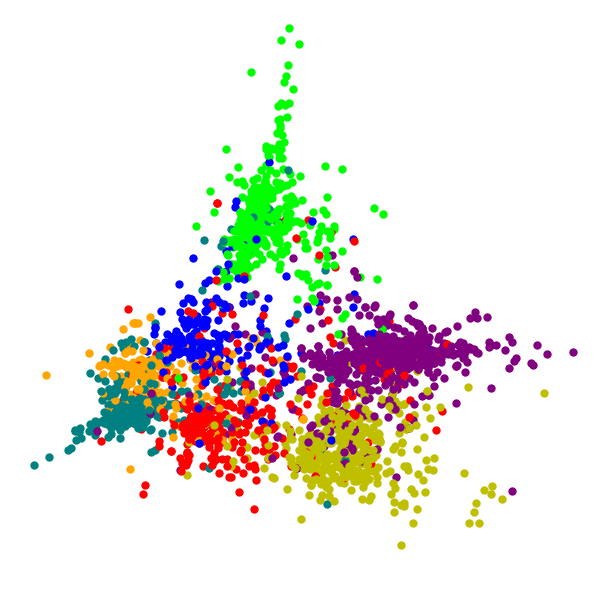}
            \label{fig:tsne-cora1}
        }
        % \hspace{0.06\textwidth}
        \subfigure[Cora $Z^{(2)}$]{
            \centering
            \includegraphics[width=0.3\linewidth]{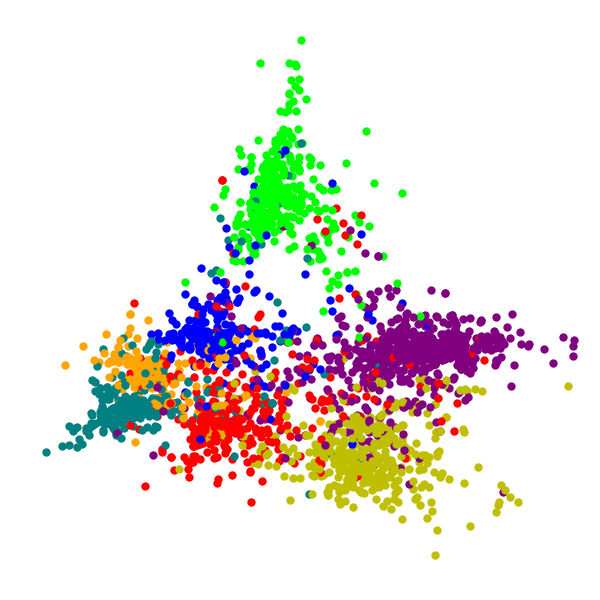}
            \label{fig:tsne-cora2}
        }
    \end{minipage}
    \hfill
    \begin{minipage}[b]{\linewidth}
        \centering
        \subfigure[Citeseer $Z^{(0)}$]{
            \centering
            \includegraphics[width=0.3\linewidth]{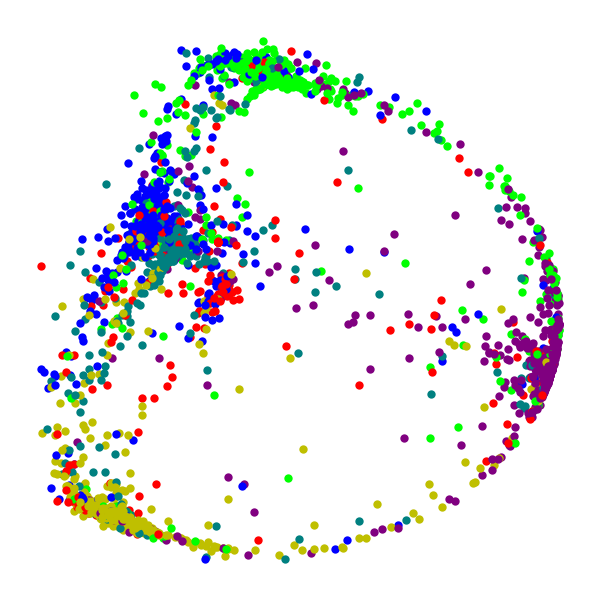}
            \label{fig:tsne-citeseer0}
        }
        % \hspace{0.06\textwidth}
        \subfigure[Citeseer $Z^{(1)}$]{
            \centering
            \includegraphics[width=0.3\linewidth]{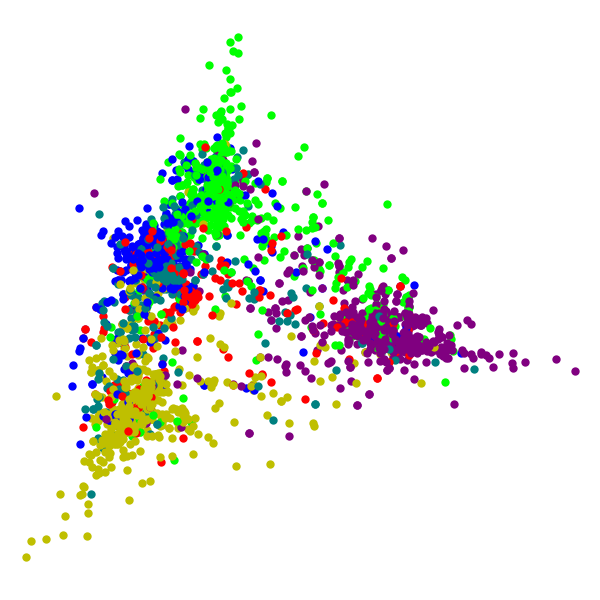}
            \label{fig:tsne-citeseer1}
        }
        % \hspace{0.06\textwidth}
        \subfigure[Citeseer $Z^{(2)}$]{
            \centering
            \includegraphics[width=0.3\linewidth]{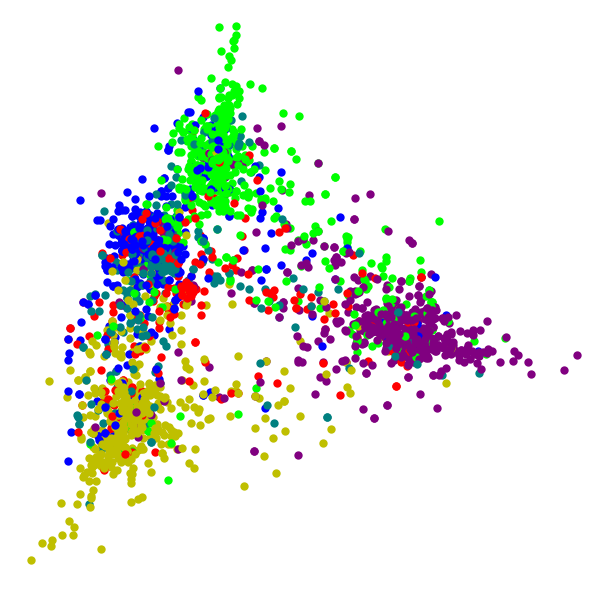}
            \label{fig:tsne-citeseer2}
        }
    \end{minipage}
    \hfill
    \begin{minipage}[b]{\linewidth}
        \centering
        \subfigure[Pubmed $Z^{(0)}$]{
            \centering
            \includegraphics[width=0.3\linewidth]{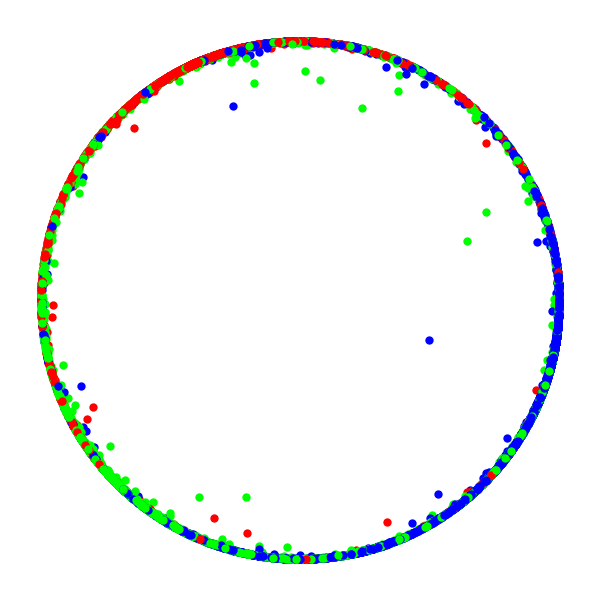}
            \label{fig:tsne-pubmed0}
        }
        % \hspace{0.06\textwidth}
        \subfigure[Pubmed $Z^{(1)}$]{
            \centering
            \includegraphics[width=0.3\linewidth]{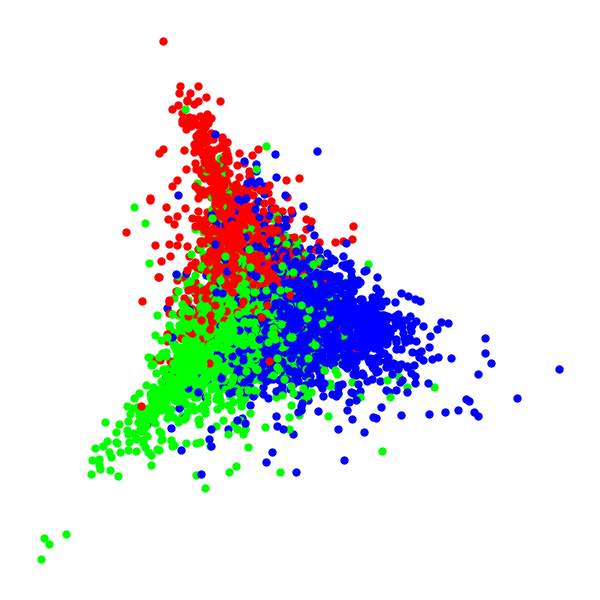}
            \label{fig:tsne-pubmed1}
        }
        % \hspace{0.06\textwidth}
        \subfigure[Pubmed $Z^{(2)}$]{
            \centering
            \includegraphics[width=0.3\linewidth]{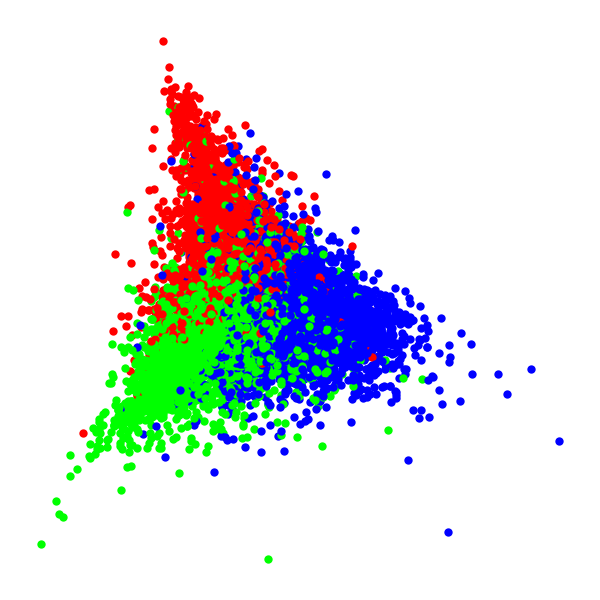}
            \label{fig:tsne-pubmed2}
        }
    \end{minipage}

    \caption{Visualization on Planetoid datasets}
    \label{fig:tsne-planetoid}
\end{figure}

\subsection{Implementation Details}
\label{sec:impl-detail}
We implement NormProp in Pytorch \cite{paszke2019pytorch} and Pytorch Geometric \cite{fey2019pyg}.
We use the two-layer MLP with hidden size in $\{32, 64, 256, 512\}$.
We tune the following hyper-parameters: $K \in \{2, 3\}$; $\lambda \in [0, 2]$; weight decay $\in \{1e-2, 5e-3, 1e-3, 5e-4, 1e-4, 0\}$; similarity threshold $\tau \in [0, 1.0]$.
Moreover, we set the dimension of hyperspherical space to $8$ for standard semi-supervised node classification, 64 for ogbn-arxiv, and $32$ for other datasets.
We set the dropout rate to $0.3$.
For obgn-arxiv, we set the warmup to $100$, and for the rest of the datasets, it is $10$.
The model is trained for 300 epochs, and the best model is selected based on the validation set.

The setup of baseline methods for datasets other than ogbn-arxiv refers to Violin \cite{ijcai2023violin} and Meta-PN \cite{aaai2022meta-pn}.
For the ogbn-arxiv \cite{hu2020ogb}, more details are as follows:
\begin{itemize}
    \item MLP: We configure the hidden size to 512 for the two-layer MLP.
    \item LP \footnote{\url{https://github.com/pyg-team/pytorch_geometric/blob/master/examples/label_prop.py}} \cite{zhu2002label-propagation}: We set the $\alpha$ to $0.1$, and $K$ to $10$.
    \item GCN  \footnote{\url{https://github.com/snap-stanford/ogb/tree/master/examples/nodeproppred/arxiv}} \cite{DBLP:conf/iclr/2017/gcn}: Following the configuration of OGB benchmark \cite{hu2020ogb}, we set the hidden size to $512$ and the layers of GCN to $3$.
    \item SGC \footnote{\url{https://github.com/Tiiiger/SGC}} \cite{icml2019sgc}: We apply the two-layer feature propagation.
    \item APPNP \footnote{\url{https://github.com/benedekrozemberczki/APPNP}} \cite{iclr2019appnp}: Following to the Meta-PN, we set the hidden size to $64$, $K$ to $10$, and $\alpha$ to $0.1$.
    \item DAGNN: \footnote{\url{https://github.com/mengliu1998/DeeperGNN}} \cite{kdd2020dagnn}: We follow the default settings provided by the authors for the best performance.
    \item C\&S \footnote{\url{https://github.com/CUAI/CorrectAndSmooth}} \cite{huang2020c-and-s}: We follow the default settings provided by the authors for the best performance.
    \item Meta-PN
    \footnote{\url{https://github.com/kaize0409/Meta-PN}} \cite{aaai2022meta-pn}: We follow the default settings provided by the authors for the best performance.
\end{itemize}

\subsection{Computational Infrastructure Details}
\label{sec:device}
All experiments in this paper are conduct on the device given in Table \ref{tab:device}.
Our code implementation relies on the deep learning framework Pytorch 2.0 \cite{paszke2019pytorch} and graph neural network library Pytorch Geometric 2.3.1 \cite{fey2019pyg}.

\begin{table}[H]
    \centering
    \resizebox{0.65\linewidth}{!}{
        \begin{tabular}{c | c}
        \toprule
        Device      & Value                 \\
        \midrule
        System      & Ubuntu 20.04          \\
        GPU         & NVIDIA Tesla V100     \\
        GPU memory  & 32G                   \\
        CUDA version& 11.8                  \\
        CPU         & Intel Xeon Gold 6248  \\
        Memory      & 128G                  \\
        \bottomrule
        \end{tabular}
    }
\caption{Computational infrastructure details.}
\label{tab:device}
\end{table}
